# Supplementary material for: Density-functional theory for systems with noncollinear spin: orbital-dependent exchange-correlation functionals and their application to the Hubbard dimer
Source: arXiv:1805.06417 ancillary file (2018-05-16)
Supplement: Supplementary file 1 [file Supplemental.pdf]

# Supplemental material for: Density-functional theory for systems with noncollinear spin: orbital-dependent exchange-correlation functionals and their application to the Hubbard dimer

Carsten A. Ullrich
*Department of Physics and Astronomy, University of Missouri, Columbia, Missouri 65211, USA*
(Dated: May 15, 2018)

## I. OEP, KLI, AND SLATER FOR NONCOLLINEAR SPINS

### A. Derivation of the OEP equation

We start from the definition of the xc potential as a functional derivative of the xc energy, see Eq. (13) of the main paper:

$$v^{\rm xc}_{\alpha\beta}(\mathbf{r}) = \frac{\delta E_{\rm xc}[\underline{\underline{n}}]}{\delta n_{\beta\alpha}(\mathbf{r})}\,, \tag{1}$$

where Greek indices denote spin ↑ or ↓. Now consider the case where the xc energy is given as an orbital functional, $E_{\rm xc}[\{\psi_{i\sigma}\}]$. To carry out the functional derivative of Eq. (1) for implicit density functionals we use the chain rule for functional differentiation:

$$\begin{aligned} v^{\rm xc}_{\alpha\beta}(\mathbf{r}) &= \sum_{\gamma\delta}\int d\mathbf{r}'\,\frac{\delta E_{\rm xc}}{\delta v_{\gamma\delta}(\mathbf{r}')}\frac{\delta v_{\gamma\delta}(\mathbf{r}')}{\delta n_{\beta\alpha}(\mathbf{r})} \\ &= \sum_i^N\sum_{\gamma\delta\tau}\int d\mathbf{r}'\int d\mathbf{r}''\,\frac{\delta E_{\rm xc}}{\delta\psi_{i\tau}(\mathbf{r}'')}\frac{\delta\psi_{i\tau}(\mathbf{r}'')}{\delta v_{\gamma\delta}(\mathbf{r}')}\frac{\delta v_{\gamma\delta}(\mathbf{r}')}{\delta n_{\beta\alpha}(\mathbf{r})} \\ &+ \sum_i^N\sum_{\gamma\delta\tau}\int d\mathbf{r}'\int d\mathbf{r}''\,\frac{\delta E_{\rm xc}}{\delta\psi^*_{i\tau}(\mathbf{r}'')}\frac{\delta\psi^*_{i\tau}(\mathbf{r}'')}{\delta v_{\gamma\delta}(\mathbf{r}')}\frac{\delta v_{\gamma\delta}(\mathbf{r}')}{\delta n_{\beta\alpha}(\mathbf{r})}\,, \end{aligned} \tag{2}$$

where $v_{\gamma\delta}(\mathbf{r})$ is the Kohn-Sham potential. Now multiply with the inverse of the last functional derivative:

$$\begin{aligned} \sum_{\alpha\beta}\int d\mathbf{r}\, v^{\rm xc}_{\alpha\beta}(\mathbf{r})\frac{\delta n_{\beta\alpha}(\mathbf{r})}{\delta v_{\mu\nu}(\mathbf{r}''')} &= \sum_i^N\sum_{\alpha\beta}\int d\mathbf{r}\sum_{\gamma\delta\tau}\int d\mathbf{r}'\int d\mathbf{r}''\,\frac{\delta E_{\rm xc}}{\delta\psi_{i\tau}(\mathbf{r}'')}\frac{\delta\psi_{i\tau}(\mathbf{r}'')}{\delta v_{\gamma\delta}(\mathbf{r}')}\frac{\delta v_{\gamma\delta}(\mathbf{r}')}{\delta n_{\beta\alpha}(\mathbf{r})}\frac{\delta n_{\beta\alpha}(\mathbf{r})}{\delta v_{\mu\nu}(\mathbf{r}''')} \\ &+ \sum_i^N\sum_{\alpha\beta}\int d\mathbf{r}\sum_{\gamma\delta\tau}\int d\mathbf{r}'\int d\mathbf{r}''\,\frac{\delta E_{\rm xc}}{\delta\psi^*_{i\tau}(\mathbf{r}'')}\frac{\delta\psi^*_{i\tau}(\mathbf{r}'')}{\delta v_{\gamma\delta}(\mathbf{r}')}\frac{\delta v_{\gamma\delta}(\mathbf{r}')}{\delta n_{\beta\alpha}(\mathbf{r})}\frac{\delta n_{\beta\alpha}(\mathbf{r})}{\delta v_{\mu\nu}(\mathbf{r}''')} \\ &= \sum_i^N\sum_\tau\int d\mathbf{r}'\left(\frac{\delta E_{\rm xc}}{\delta\psi_{i\tau}(\mathbf{r}')}\frac{\delta\psi_{i\tau}(\mathbf{r}')}{\delta v_{\mu\nu}(\mathbf{r}''')} + \frac{\delta E_{\rm xc}}{\delta\psi^*_{i\tau}(\mathbf{r}')}\frac{\delta\psi^*_{i\tau}(\mathbf{r}')}{\delta v_{\mu\nu}(\mathbf{r}''')}\right). \end{aligned} \tag{3}$$

We have

$$\frac{\delta n_{\beta\alpha}(\mathbf{r}')}{\delta v_{\mu\nu}(\mathbf{r})} = \sum_i^N\left(\psi_{i\beta}(\mathbf{r}')\frac{\delta\psi^*_{i\alpha}(\mathbf{r}')}{\delta v_{\mu\nu}(\mathbf{r})} + \psi^*_{i\alpha}(\mathbf{r}')\frac{\delta\psi_{i\beta}(\mathbf{r}')}{\delta v_{\mu\nu}(\mathbf{r})}\right). \tag{4}$$

This can now be put together as follows:

$$\begin{aligned} 0 &= \sum_i^N\sum_{\alpha\beta}\int d\mathbf{r}'\, v^{\rm xc}_{\alpha\beta}(\mathbf{r}')\left(\psi_{i\beta}(\mathbf{r}')\frac{\delta\psi^*_{i\alpha}(\mathbf{r}')}{\delta v_{\mu\nu}(\mathbf{r})} + \psi^*_{i\alpha}(\mathbf{r}')\frac{\delta\psi_{i\beta}(\mathbf{r}')}{\delta v_{\mu\nu}(\mathbf{r})}\right) \\ &- \sum_i^N\sum_\tau\int d\mathbf{r}'\left(\frac{\delta E_{\rm xc}}{\delta\psi_{i\tau}(\mathbf{r}')}\frac{\delta\psi_{i\tau}(\mathbf{r}')}{\delta v_{\mu\nu}(\mathbf{r})} + \frac{\delta E_{\rm xc}}{\delta\psi^*_{i\tau}(\mathbf{r}')}\frac{\delta\psi^*_{i\tau}(\mathbf{r}')}{\delta v_{\mu\nu}(\mathbf{r})}\right) \\ &= \sum_i^N\int d\mathbf{r}'\left[\left(\sum_{\alpha\beta}v^{\rm xc}_{\alpha\beta}(\mathbf{r}')\psi_{i\beta}(\mathbf{r}') - \sum_\alpha\frac{\delta E_{\rm xc}}{\delta\psi^*_{i\alpha}(\mathbf{r}')}\right)\frac{\delta\psi^*_{i\alpha}(\mathbf{r}')}{\delta v_{\mu\nu}(\mathbf{r})}\right] \\ &+ \sum_i^N\int d\mathbf{r}'\left[\left(\sum_{\alpha\beta}v^{\rm xc}_{\alpha\beta}(\mathbf{r}')\psi^*_{i\alpha}(\mathbf{r}') - \sum_\beta\frac{\delta E_{\rm xc}}{\delta\psi_{i\beta}(\mathbf{r}')}\right)\frac{\delta\psi_{i\beta}(\mathbf{r}')}{\delta v_{\mu\nu}(\mathbf{r})}\right]. \end{aligned} \tag{5}$$

We have from first-order perturbation theory

$$\frac{\delta\psi_{i\beta}(\mathbf{r}')}{\delta v_{\mu\nu}(\mathbf{r})} = -\sum_{j\neq i}^{\infty} \frac{\psi^*_{j\mu}(\mathbf{r})\psi_{i\nu}(\mathbf{r})\psi_{j\beta}(\mathbf{r}')}{\epsilon_j - \epsilon_i}\,, \qquad \frac{\delta\psi^*_{i\alpha}(\mathbf{r}')}{\delta v_{\mu\nu}(\mathbf{r})} = -\sum_{j\neq i}^{\infty} \frac{\psi^*_{i\mu}(\mathbf{r})\psi_{j\nu}(\mathbf{r})\psi^*_{j\alpha}(\mathbf{r}')}{\epsilon_j - \epsilon_i} \tag{6}$$

for which we used $v_{\uparrow\downarrow} = v^*_{\downarrow\uparrow}$. This gives the OEP equation, Eq. (20) in the main text, as follows:

$$\begin{aligned} 0 = &\sum_i^N \sum_{j\neq i}^{\infty} \int d\mathbf{r}' \left( \sum_{\alpha\beta} v^{\rm xc}_{\alpha\beta}(\mathbf{r}')\psi_{i\beta}(\mathbf{r}') - \sum_\alpha \frac{\delta E_{\rm xc}}{\delta\psi^*_{i\alpha}(\mathbf{r}')}\right) \frac{\psi^*_{i\mu}(\mathbf{r})\psi_{j\nu}(\mathbf{r})\psi^*_{j\alpha}(\mathbf{r}')}{\epsilon_j - \epsilon_i} \\ &+ \sum_i^N \sum_{j\neq i}^{\infty} \int d\mathbf{r}' \left( \sum_{\alpha\beta} v^{\rm xc}_{\alpha\beta}(\mathbf{r}')\psi^*_{i\alpha}(\mathbf{r}') - \sum_\beta \frac{\delta E_{\rm xc}}{\delta\psi_{i\beta}(\mathbf{r}')}\right) \frac{\psi^*_{j\mu}(\mathbf{r})\psi_{i\nu}(\mathbf{r})\psi_{j\beta}(\mathbf{r}')}{\epsilon_j - \epsilon_i}\,. \end{aligned} \tag{7}$$

### B. Derivation of the KLI approximation

To obtain the KLI approximation, we replace the energy denominators in the OEP equation, Eq. (7), by some average constant $\bar{\epsilon}$, which can then be canceled out. The result is as follows:

$$\begin{aligned} 0 = &\sum_i^N \sum_{j\neq i}^{\infty} \int d\mathbf{r}' \left( \sum_{\alpha\beta} v^{\rm xcK}_{\alpha\beta}(\mathbf{r}')\psi_{i\beta}(\mathbf{r}') - \sum_\alpha \frac{\delta E_{\rm xc}}{\delta\psi^*_{i\alpha}(\mathbf{r}')}\right) \psi^*_{i\mu}(\mathbf{r})\psi_{j\nu}(\mathbf{r})\psi^*_{j\alpha}(\mathbf{r}') \\ &+ \sum_i^N \sum_{j\neq i}^{\infty} \int d\mathbf{r}' \left( \sum_{\alpha\beta} v^{\rm xcK}_{\alpha\beta}(\mathbf{r}')\psi^*_{i\alpha}(\mathbf{r}') - \sum_\beta \frac{\delta E_{\rm xc}}{\delta\psi_{i\beta}(\mathbf{r}')}\right) \psi^*_{j\mu}(\mathbf{r})\psi_{i\nu}(\mathbf{r})\psi_{j\beta}(\mathbf{r}')\,. \end{aligned} \tag{8}$$

We write this as

$$\begin{aligned} 0 = &\sum_i^N \sum_{j}^{\infty} \int d\mathbf{r}' \left( \sum_{\alpha\beta} v^{\rm xcK}_{\alpha\beta}(\mathbf{r}')\psi_{i\beta}(\mathbf{r}') - \sum_\alpha \frac{\delta E_{\rm xc}}{\delta\psi^*_{i\alpha}(\mathbf{r}')}\right) \psi^*_{i\mu}(\mathbf{r})\psi_{j\nu}(\mathbf{r})\psi^*_{j\alpha}(\mathbf{r}') \\ &+ \sum_i^N \sum_{j}^{\infty} \int d\mathbf{r}' \left( \sum_{\alpha\beta} v^{\rm xcK}_{\alpha\beta}(\mathbf{r}')\psi^*_{i\alpha}(\mathbf{r}') - \sum_\beta \frac{\delta E_{\rm xc}}{\delta\psi_{i\beta}(\mathbf{r}')}\right) \psi^*_{j\mu}(\mathbf{r})\psi_{i\nu}(\mathbf{r})\psi_{j\beta}(\mathbf{r}') \\ &- \sum_i^N \int d\mathbf{r}' \left( \sum_{\alpha\beta} v^{\rm xcK}_{\alpha\beta}(\mathbf{r}')\psi_{i\beta}(\mathbf{r}') - \sum_\alpha \frac{\delta E_{\rm xc}}{\delta\psi^*_{i\alpha}(\mathbf{r}')}\right) \psi^*_{i\mu}(\mathbf{r})\psi_{i\nu}(\mathbf{r})\psi^*_{i\alpha}(\mathbf{r}') \\ &- \sum_i^N \int d\mathbf{r}' \left( \sum_{\alpha\beta} v^{\rm xcK}_{\alpha\beta}(\mathbf{r}')\psi^*_{i\alpha}(\mathbf{r}') - \sum_\beta \frac{\delta E_{\rm xc}}{\delta\psi_{i\beta}(\mathbf{r}')}\right) \psi^*_{i\mu}(\mathbf{r})\psi_{i\nu}(\mathbf{r})\psi_{i\beta}(\mathbf{r}'). \end{aligned} \tag{9}$$

The completeness relation is

$$\sum_j^{\infty} \Psi_j(\mathbf{r})\Psi^\dagger_j(\mathbf{r}') = \underline{\underline{1}}\,\delta(\mathbf{r}-\mathbf{r}') \tag{10}$$

or, component by component,

$$\begin{aligned} \sum_j \psi_{j\uparrow}(\mathbf{r})\psi^*_{j\uparrow}(\mathbf{r}') &= \sum_j \psi_{j\downarrow}(\mathbf{r})\psi^*_{j\downarrow}(\mathbf{r}') = \delta(\mathbf{r}-\mathbf{r}') \\ \sum_j \psi_{j\uparrow}(\mathbf{r})\psi^*_{j\downarrow}(\mathbf{r}') &= \sum_j \psi_{j\downarrow}(\mathbf{r})\psi^*_{j\uparrow}(\mathbf{r}') = 0\,. \end{aligned} \tag{11}$$

This gives

$$
\begin{aligned}
0 &= \sum_i^N \int d\mathbf{r}' \left( \sum_{\alpha\beta} v^{\mathrm{xcK}}_{\alpha\beta}(\mathbf{r}')\psi_{i\beta}(\mathbf{r}') - \sum_\alpha \frac{\delta E_{\mathrm{xc}}}{\delta \psi^*_{i\alpha}(\mathbf{r}')} \right) \psi^*_{i\mu}(\mathbf{r})\delta(\mathbf{r}-\mathbf{r}')\delta_{\nu\alpha} \\
&+ \sum_i^N \int d\mathbf{r}' \left( \sum_{\alpha\beta} v^{\mathrm{xcK}}_{\alpha\beta}(\mathbf{r}')\psi^*_{i\alpha}(\mathbf{r}') - \sum_\beta \frac{\delta E_{\mathrm{xc}}}{\delta \psi_{i\beta}(\mathbf{r}')} \right) \psi_{i\nu}(\mathbf{r})\delta(\mathbf{r}-\mathbf{r}')\delta_{\mu\beta} \\
&- \sum_i^N \int d\mathbf{r}' \left( \sum_{\alpha\beta} v^{\mathrm{xcK}}_{\alpha\beta}(\mathbf{r}')\psi_{i\beta}(\mathbf{r}') - \sum_\alpha \frac{\delta E_{\mathrm{xc}}}{\delta \psi^*_{i\alpha}(\mathbf{r}')} \right) \psi^*_{i\mu}(\mathbf{r})\psi_{i\nu}(\mathbf{r})\psi^*_{i\alpha}(\mathbf{r}') \\
&- \sum_i^N \int d\mathbf{r}' \left( \sum_{\alpha\beta} v^{\mathrm{xcK}}_{\alpha\beta}(\mathbf{r}')\psi^*_{i\alpha}(\mathbf{r}') - \sum_\beta \frac{\delta E_{\mathrm{xc}}}{\delta \psi_{i\beta}(\mathbf{r}')} \right) \psi^*_{i\mu}(\mathbf{r})\psi_{i\nu}(\mathbf{r})\psi_{i\beta}(\mathbf{r}') \\
&= \sum_i^N \left( \sum_\beta v^{\mathrm{xcK}}_{\nu\beta}(\mathbf{r})\psi_{i\beta}(\mathbf{r}) - \frac{\delta E_{\mathrm{xc}}}{\delta \psi^*_{i\nu}(\mathbf{r})} \right) \psi^*_{i\mu}(\mathbf{r}) + \sum_i^N \left( \sum_\alpha v^{\mathrm{xcK}}_{\alpha\mu}(\mathbf{r})\psi^*_{i\alpha}(\mathbf{r}) - \frac{\delta E_{\mathrm{xc}}}{\delta \psi_{i\mu}(\mathbf{r})} \right) \psi_{i\nu}(\mathbf{r}) \\
&- \sum_i^N \int d\mathbf{r}' \left( \sum_{\alpha\beta} v^{\mathrm{xcK}}_{\alpha\beta}(\mathbf{r}')\psi_{i\beta}(\mathbf{r}')\psi^*_{i\alpha}(\mathbf{r}') - \sum_\alpha \frac{\delta E_{\mathrm{xc}}}{\delta \psi^*_{i\alpha}(\mathbf{r}')}\psi^*_{i\alpha}(\mathbf{r}') \right) \psi^*_{i\mu}(\mathbf{r})\psi_{i\nu}(\mathbf{r}) \\
&- \sum_i^N \int d\mathbf{r}' \left( \sum_{\alpha\beta} v^{\mathrm{xcK}}_{\alpha\beta}(\mathbf{r}')\psi^*_{i\alpha}(\mathbf{r}')\psi_{i\beta}(\mathbf{r}') - \sum_\beta \frac{\delta E_{\mathrm{xc}}}{\delta \psi_{i\beta}(\mathbf{r}')}\psi_{i\beta}(\mathbf{r}') \right) \psi^*_{i\mu}(\mathbf{r})\psi_{i\nu}(\mathbf{r})
\end{aligned} \tag{12}
$$

which can also be written as

$$
\begin{aligned}
0 &= \sum_\alpha \left[ v^{\mathrm{xcK}}_{\nu\alpha}(\mathbf{r})n_{\alpha\mu}(\mathbf{r}) + n_{\nu\alpha}(\mathbf{r})v^{\mathrm{xcK}}_{\alpha\mu}(\mathbf{r}) \right] - \sum_i^N \left( \frac{\delta E_{\mathrm{xc}}}{\delta \psi^*_{i\nu}(\mathbf{r})}\psi^*_{i\mu}(\mathbf{r}) + \frac{\delta E_{\mathrm{xc}}}{\delta \psi_{i\mu}(\mathbf{r})}\psi_{i\nu}(\mathbf{r}) \right) \\
&- \sum_i^N \int d\mathbf{r}' \left( \sum_{\alpha\beta} v^{\mathrm{xcK}}_{\alpha\beta}(\mathbf{r}')\psi_{i\beta}(\mathbf{r}')\psi^*_{i\alpha}(\mathbf{r}') - \sum_\alpha \frac{\delta E_{\mathrm{xc}}}{\delta \psi^*_{i\alpha}(\mathbf{r}')}\psi^*_{i\alpha}(\mathbf{r}') \right) \psi^*_{i\mu}(\mathbf{r})\psi_{i\nu}(\mathbf{r}) \\
&- \sum_i^N \int d\mathbf{r}' \left( \sum_{\alpha\beta} v^{\mathrm{xcK}}_{\alpha\beta}(\mathbf{r}')\psi^*_{i\alpha}(\mathbf{r}')\psi_{i\beta}(\mathbf{r}') - \sum_\beta \frac{\delta E_{\mathrm{xc}}}{\delta \psi_{i\beta}(\mathbf{r}')}\psi_{i\beta}(\mathbf{r}') \right) \psi^*_{i\mu}(\mathbf{r})\psi_{i\nu}(\mathbf{r})\,.
\end{aligned} \tag{13}
$$

We thus end up with the KLI equation, Eq. (21) in the main paper:

$$
\begin{aligned}
\left[\underline{\underline{v}}^{\mathrm{xcK}}\underline{\underline{n}}\right]_{\nu\mu} + \left[\underline{\underline{n}}\,\underline{\underline{v}}^{\mathrm{xcK}}\right]_{\nu\mu} &= \sum_i^N \left( \frac{\delta E_{\mathrm{xc}}}{\delta \psi^*_{i\nu}(\mathbf{r})}\psi^*_{i\mu}(\mathbf{r}) + \frac{\delta E_{\mathrm{xc}}}{\delta \psi_{i\mu}(\mathbf{r})}\psi_{i\nu}(\mathbf{r}) \right) \\
&+ \sum_i^N \int d\mathbf{r}' \left( \sum_{\alpha\beta} v^{\mathrm{xcK}}_{\alpha\beta}(\mathbf{r}')\psi_{i\beta}(\mathbf{r}')\psi^*_{i\alpha}(\mathbf{r}') - \sum_\alpha \frac{\delta E_{\mathrm{xc}}}{\delta \psi^*_{i\alpha}(\mathbf{r}')}\psi^*_{i\alpha}(\mathbf{r}') \right) \psi^*_{i\mu}(\mathbf{r})\psi_{i\nu}(\mathbf{r}) \\
&+ \sum_i^N \int d\mathbf{r}' \left( \sum_{\alpha\beta} v^{\mathrm{xcK}}_{\alpha\beta}(\mathbf{r}')\psi^*_{i\alpha}(\mathbf{r}')\psi_{i\beta}(\mathbf{r}') - \sum_\beta \frac{\delta E_{\mathrm{xc}}}{\delta \psi_{i\beta}(\mathbf{r}')}\psi_{i\beta}(\mathbf{r}') \right) \psi^*_{i\mu}(\mathbf{r})\psi_{i\nu}(\mathbf{r})\,.
\end{aligned} \tag{14}
$$

Now let us consider the special case of exchange-only. The exchange energy is given by

$$
E_{\mathrm{x}} = -\frac{1}{2}\sum_{\sigma\tau} \iint \frac{d\mathbf{r}d\mathbf{r}'}{|\mathbf{r}-\mathbf{r}'|}\gamma_{\sigma\tau}(\mathbf{r},\mathbf{r}')\gamma_{\tau\sigma}(\mathbf{r}',\mathbf{r}), \tag{15}
$$

where the spin-resolved reduced 1-particle Kohn-Sham density matrix is

$$
\gamma_{\sigma\tau}(\mathbf{r},\mathbf{r}') = \sum_j^N \psi_{j\sigma}(\mathbf{r})\psi^*_{j\tau}(\mathbf{r}'). \tag{16}
$$

The functional derivative of the exchange energy with respect to the orbitals is

$$\frac{\delta E_{\rm x}}{\delta\psi^*_{i\nu}(\mathbf{r})} = -\sum_j^N\sum_\tau\int\frac{d\mathbf{r}'}{|\mathbf{r}-\mathbf{r}'|}\psi^*_{j\tau}(\mathbf{r}')\psi_{i\tau}(\mathbf{r}')\psi_{j\nu}(\mathbf{r})$$
$$\frac{\delta E_{\rm x}}{\delta\psi_{i\mu}(\mathbf{r})} = -\sum_j^N\sum_\tau\int\frac{d\mathbf{r}'}{|\mathbf{r}-\mathbf{r}'|}\psi_{j\tau}(\mathbf{r}')\psi^*_{i\tau}(\mathbf{r}')\psi^*_{j\mu}(\mathbf{r})\,.$$

Plugging this into Eq. (14) gives

$$\begin{aligned}
&\left[\underline{\underline{v}}^{\rm xK}(\mathbf{r})\underline{\underline{n}}(\mathbf{r})\right]_{\nu\mu} + \left[\underline{\underline{n}}(\mathbf{r})\underline{\underline{v}}^{\rm xK}(\mathbf{r})\right]_{\nu\mu}\\
&= -\sum_{ij}^N\sum_\tau\int\frac{d\mathbf{r}'}{|\mathbf{r}-\mathbf{r}'|}\left(\psi^*_{j\tau}(\mathbf{r}')\psi_{i\tau}(\mathbf{r}')\psi_{j\nu}(\mathbf{r})\psi^*_{i\mu}(\mathbf{r}) + \psi_{j\tau}(\mathbf{r}')\psi^*_{i\tau}(\mathbf{r}')\psi^*_{j\mu}(\mathbf{r})\psi_{i\nu}(\mathbf{r})\right)\\
&+\sum_i^N\int d\mathbf{r}'\left(\sum_{\alpha\beta}v^{\rm xK}_{\alpha\beta}(\mathbf{r}')n_{i,\beta\alpha}(\mathbf{r}') + \sum_j^N\sum_{\tau\alpha}\int\frac{d\mathbf{r}''}{|\mathbf{r}'-\mathbf{r}''|}\psi^*_{j\tau}(\mathbf{r}'')\psi_{i\tau}(\mathbf{r}'')\psi_{j\alpha}(\mathbf{r}')\psi^*_{i\alpha}(\mathbf{r}')\right)n_{i,\nu\mu}(\mathbf{r})\\
&+\sum_i^N\int d\mathbf{r}'\left(\sum_{\alpha\beta}v^{\rm xK}_{\alpha\beta}(\mathbf{r}')n_{i,\beta\alpha}(\mathbf{r}') + \sum_j^N\sum_{\tau\alpha}\int\frac{d\mathbf{r}''}{|\mathbf{r}'-\mathbf{r}''|}\psi_{j\tau}(\mathbf{r}'')\psi^*_{i\tau}(\mathbf{r}'')\psi^*_{j\alpha}(\mathbf{r}')\psi_{i\alpha}(\mathbf{r}')\right)n_{i,\nu\mu}(\mathbf{r})\\
&= -2\sum_\tau\int\frac{d\mathbf{r}'}{|\mathbf{r}-\mathbf{r}'|}\gamma_{\nu\tau}(\mathbf{r},\mathbf{r}')\gamma_{\tau\mu}(\mathbf{r}',\mathbf{r})\\
&+2\sum_i^N\int d\mathbf{r}'\left(\sum_{\alpha\beta}v^{\rm xK}_{\alpha\beta}(\mathbf{r}')n_{i,\beta\alpha}(\mathbf{r}') + \sum_{\tau\alpha}\int\frac{d\mathbf{r}''}{|\mathbf{r}'-\mathbf{r}''|}\gamma_{\alpha\tau}(\mathbf{r}',\mathbf{r}'')\psi^*_{i\alpha}(\mathbf{r}')\psi_{i\tau}(\mathbf{r}'')\right)n_{i,\nu\mu}(\mathbf{r})\\
&= -2\int\frac{d\mathbf{r}'}{|\mathbf{r}-\mathbf{r}'|}\left[\underline{\underline{\gamma}}(\mathbf{r},\mathbf{r}')\underline{\underline{\gamma}}(\mathbf{r}',\mathbf{r})\right]_{\nu\mu}\\
&+2\sum_i^N\int d\mathbf{r}'\left(\mathrm{tr}\,\underline{\underline{v}}^{\rm xK}(\mathbf{r}')\underline{\underline{n_i}}(\mathbf{r}') + \int\frac{d\mathbf{r}''}{|\mathbf{r}'-\mathbf{r}''|}\mathrm{tr}\,\underline{\underline{\gamma}}(\mathbf{r}',\mathbf{r}'')\underline{\underline{\gamma_i}}(\mathbf{r}'',\mathbf{r}')\right)n_{i,\nu\mu}(\mathbf{r})
\end{aligned}\tag{17}$$

and we can write this as

$$\begin{aligned}
\underline{\underline{v}}^{\rm xK}(\mathbf{r})\underline{\underline{n}}(\mathbf{r}) + \underline{\underline{n}}(\mathbf{r})\underline{\underline{v}}^{\rm xK}(\mathbf{r}) = &-2\int\frac{d\mathbf{r}'}{|\mathbf{r}-\mathbf{r}'|}\,\underline{\underline{\gamma}}(\mathbf{r},\mathbf{r}')\underline{\underline{\gamma}}(\mathbf{r}',\mathbf{r})\\
&+2\sum_i^N\underline{\underline{n_i}}(\mathbf{r})\int d\mathbf{r}'\left(\mathrm{tr}\,\underline{\underline{v}}^{\rm xK}(\mathbf{r}')\underline{\underline{n_i}}(\mathbf{r}') + \int\frac{d\mathbf{r}''}{|\mathbf{r}'-\mathbf{r}''|}\mathrm{tr}\,\underline{\underline{\gamma}}(\mathbf{r}',\mathbf{r}'')\underline{\underline{\gamma_i}}(\mathbf{r}'',\mathbf{r}')\right).
\end{aligned}\tag{18}$$

This is the generalization of the original KLI exchange potential by Krieger et al.[1]

### C. Slater potential

To get the Slater potential from the KLI approximation, we throw away the orbital-dependent constants, i.e., the second and third line in Eq. (14). This gives

$$\left[\underline{\underline{v}}^{\rm xcS}\underline{\underline{n}}\right]_{\nu\mu} + \left[\underline{\underline{n}}\,\underline{\underline{v}}^{\rm xcS}\right]_{\nu\mu} = \sum_i^N\left(\frac{\delta E_{\rm xc}}{\delta\psi^*_{i\nu}(\mathbf{r})}\psi^*_{i\mu}(\mathbf{r}) + \frac{\delta E_{\rm xc}}{\delta\psi_{i\mu}(\mathbf{r})}\psi_{i\nu}(\mathbf{r})\right) \equiv b_{\nu\mu}\,. \tag{19}$$

This means we need to solve the following matrix equation, see Eq. (24) of the main paper:

$$\underline{\underline{v}}^{\rm xcS}\,\underline{\underline{n}} + \underline{\underline{n}}\,\underline{\underline{v}}^{\rm xcS} = \underline{\underline{b}}. \tag{20}$$

This has the form of a so-called Sylvester equation. The solution cannot be easily expressed as a $2\times2$ matrix, but it can be done in a slightly different way, using a $4\times4$ matrix-vector notation. Using $n = n_{\uparrow\uparrow} + n_{\downarrow\downarrow}$, the system (20)

can be written as

$$\begin{pmatrix} 2n_{\uparrow\uparrow} & n_{\uparrow\downarrow} & n_{\downarrow\uparrow} & 0 \\ n_{\downarrow\uparrow} & n & 0 & n_{\downarrow\uparrow} \\ n_{\uparrow\downarrow} & 0 & n & n_{\uparrow\downarrow} \\ 0 & n_{\uparrow\downarrow} & n_{\downarrow\uparrow} & 2n_{\downarrow\downarrow} \end{pmatrix} \begin{pmatrix} v_{\uparrow\uparrow} \\ v_{\downarrow\uparrow} \\ v_{\uparrow\downarrow} \\ v_{\downarrow\downarrow} \end{pmatrix} = \begin{pmatrix} b_{\uparrow\uparrow} \\ b_{\downarrow\uparrow} \\ b_{\uparrow\downarrow} \\ b_{\downarrow\downarrow} \end{pmatrix}. \tag{21}$$

Defining $D = n_{\uparrow\uparrow}n_{\downarrow\downarrow} - n_{\uparrow\downarrow}n_{\downarrow\uparrow}$, the solution is given by

$$\begin{pmatrix} v_{\uparrow\uparrow} \\ v_{\downarrow\uparrow} \\ v_{\uparrow\downarrow} \\ v_{\downarrow\downarrow} \end{pmatrix} = \frac{1}{2nD} \begin{pmatrix} nn_{\downarrow\downarrow} - n_{\uparrow\downarrow}n_{\downarrow\uparrow} & -n_{\downarrow\downarrow}n_{\uparrow\downarrow} & -n_{\downarrow\downarrow}n_{\downarrow\uparrow} & n_{\uparrow\downarrow}n_{\downarrow\uparrow} \\ -n_{\downarrow\downarrow}n_{\downarrow\uparrow} & 2n_{\uparrow\uparrow}n_{\downarrow\downarrow} - n_{\uparrow\downarrow}n_{\downarrow\uparrow} & n_{\downarrow\uparrow}^2 & -n_{\uparrow\uparrow}n_{\downarrow\uparrow} \\ -n_{\downarrow\downarrow}n_{\uparrow\downarrow} & n_{\uparrow\downarrow}^2 & 2n_{\uparrow\uparrow}n_{\downarrow\downarrow} - n_{\uparrow\downarrow}n_{\downarrow\uparrow} & -n_{\uparrow\uparrow}n_{\uparrow\downarrow} \\ n_{\uparrow\downarrow}n_{\downarrow\uparrow} & -n_{\uparrow\uparrow}n_{\uparrow\downarrow} & -n_{\uparrow\uparrow}n_{\downarrow\uparrow} & nn_{\uparrow\uparrow} - n_{\uparrow\downarrow}n_{\downarrow\uparrow} \end{pmatrix} \begin{pmatrix} b_{\uparrow\uparrow} \\ b_{\downarrow\uparrow} \\ b_{\uparrow\downarrow} \\ b_{\downarrow\downarrow} \end{pmatrix}. \tag{22}$$

We can define the vectorization operator **vec**, which converts an $m \times m$ matrix into a column vector of length $m^2$ by putting successive rows on top of each other. In our case

$$\mathbf{vec}\{\underline{\underline{v}}\} = \begin{pmatrix} v_{\uparrow\uparrow} \\ v_{\downarrow\uparrow} \\ v_{\uparrow\downarrow} \\ v_{\downarrow\downarrow} \end{pmatrix}$$

and similar for all other $2 \times 2$ matrices. We then define the Kronecker product notation $\otimes$, where a product of two $2 \times 2$ matrices yields a $4 \times 4$ matrix:

$$\begin{pmatrix} a_{11} & a_{12} \\ a_{21} & a_{22} \end{pmatrix} \otimes \begin{pmatrix} c_{11} & c_{12} \\ c_{21} & c_{22} \end{pmatrix} = \begin{pmatrix} a_{11}\begin{pmatrix} c_{11} & c_{12} \\ c_{21} & c_{22} \end{pmatrix} & a_{12}\begin{pmatrix} c_{11} & c_{12} \\ c_{21} & c_{22} \end{pmatrix} \\ a_{21}\begin{pmatrix} c_{11} & c_{12} \\ c_{21} & c_{22} \end{pmatrix} & a_{22}\begin{pmatrix} c_{11} & c_{12} \\ c_{21} & c_{22} \end{pmatrix} \end{pmatrix}.$$

With this notation, Eq. (20) can be recast as

$$(\underline{\underline{I}} \otimes \underline{\underline{n}} + \underline{\underline{n}}^T \otimes \underline{\underline{I}})\, \mathbf{vec}\{\underline{\underline{v}}^{\rm xcS}\} = \mathbf{vec}\{\underline{\underline{b}}\}, \tag{23}$$

where $\underline{\underline{I}}$ is the $2 \times 2$ unit matrix (in the main paper we use the notation $\underline{\underline{I}} = \sigma_0$). It is easy to see that this gives Eq. (21). We can therefore express the solution (22) formally as

$$\mathbf{vec}\{\underline{\underline{v}}^{\rm xcS}\} = (\underline{\underline{I}} \otimes \underline{\underline{n}} + \underline{\underline{n}}^T \otimes \underline{\underline{I}})^{-1}\, \mathbf{vec}\{\underline{\underline{b}}\}. \tag{24}$$

Defining

$$\underline{\underline{\mathcal{N}}} = \underline{\underline{I}} \otimes \underline{\underline{n}} + \underline{\underline{n}}^T \otimes \underline{\underline{I}}\,, \tag{25}$$

we write this in a compact manner as

$$\mathbf{vec}\{\underline{\underline{v}}^{\rm xcS}\} = \underline{\underline{\mathcal{N}}}^{-1}\, \mathbf{vec}\{\underline{\underline{b}}\}\,, \tag{26}$$

see Eq. (25) of the main paper.

## II. DERIVATION OF THE PGG EXCHANGE KERNEL

### A. Symmetry properties

We here consider only adiabatic xc kernels (i.e., no frequency dependence). The definition is

$$f^{\rm xc}_{\alpha\beta,\sigma\tau}(\mathbf{r},\mathbf{r}') = \frac{\delta^2 E_{\rm xc}}{\delta n_{\beta\alpha}(\mathbf{r})\delta n_{\sigma\tau}(\mathbf{r}')}\,. \tag{27}$$

The complex conjugate of this is

$$\left[f^{\rm xc}_{\alpha\beta,\sigma\tau}(\mathbf{r},\mathbf{r}')\right]^* = \frac{\delta^2 E_{\rm xc}}{\delta n^*_{\beta\alpha}(\mathbf{r})\delta n^*_{\sigma\tau}(\mathbf{r}')} = \frac{\delta^2 E_{\rm xc}}{\delta n_{\alpha\beta}(\mathbf{r})\delta n_{\tau\sigma}(\mathbf{r}')}$$

and therefore

$$\left[f^{\rm xc}_{\alpha\beta,\sigma\tau}(\mathbf{r},\mathbf{r}')\right]^* = f^{\rm xc}_{\beta\alpha,\tau\sigma}(\mathbf{r},\mathbf{r}')\,. \tag{28}$$

If we interchange $\mathbf{r}$ and $\mathbf{r}'$ in (27), we get

$$f^{\rm xc}_{\alpha\beta,\sigma\tau}(\mathbf{r}',\mathbf{r}) = \frac{\delta^2 E_{\rm xc}}{\delta n_{\beta\alpha}(\mathbf{r}')\delta n_{\sigma\tau}(\mathbf{r})}\,,$$

but it doesn't matter which functional derivative is taken first, so we get the condition

$$f^{\rm xc}_{\alpha\beta,\sigma\tau}(\mathbf{r}',\mathbf{r}) = f^{\rm xc}_{\tau\sigma,\beta\alpha}(\mathbf{r},\mathbf{r}'). \tag{29}$$

### B. Derivation of the kernel

To derive an orbital-dependent xc kernel, we could start from the definition (27), using an approximation for the xc energy functional. Here, however, we use a different approach, following Petersilka, Gossmann and Gross (PGG).[2,3] The so-called PGG kernel is derived making two approximations, which will be discussed in the following two subsections:

### 1. Slater approximation of the xc kernel

We define the xc kernel in a manner that is analogous to that of the Slater xc potential, see Eq. (19):

$$
\begin{aligned}
&\left[\underline{\underline{f}}^{\rm xcS}\underline{\underline{n}}\right]_{\sigma\sigma',\alpha'\alpha} + \left[\underline{\underline{n}}\,\underline{\underline{f}}^{\rm xcS}\right]_{\sigma\sigma',\alpha'\alpha} \\
&= \sum_i^N \frac{\delta v^{\rm xc}_{\sigma\sigma'}(\mathbf{r})}{\delta\psi^*_{i\alpha'}(\mathbf{r}')}\,\psi^*_{i\alpha}(\mathbf{r}') + \sum_i^N \frac{\delta v^{\rm xc}_{\sigma\sigma'}(\mathbf{r})}{\delta\psi_{i\alpha}(\mathbf{r}')}\,\psi_{i\alpha'}(\mathbf{r}') \\
&\equiv R_{\sigma\sigma',\alpha\alpha'}\ .
\end{aligned}
\qquad (30)
$$

Notice that in the second line the indices $\alpha$ and $\alpha'$ in the two functional derivatives are interchanged. This is deliberate, and takes account of the fact that the xc potential was defined in Eq. (1) using a functional derivative with respect to the transpose of the density matrix. But the second functional derivative in the definition of the xc kernel (27) is just the derivative with respect to the density matrix, not the transpose.

Now consider the left-hand side of Eq. (30). We have

$$
\begin{aligned}
&\left[\underline{\underline{f}}^{\rm xcS}\underline{\underline{n}}\right]_{\sigma\sigma',\alpha'\alpha} + \left[\underline{\underline{n}}\,\underline{\underline{f}}^{\rm xcS}\right]_{\sigma\sigma',\alpha'\alpha} \\
&= \left[\underline{\underline{f}}^{\rm xcS}\underline{\underline{n}}^T\right]_{\sigma\sigma',\alpha\alpha'} + \left[\underline{\underline{n}}^T\,\underline{\underline{f}}^{\rm xcS}\right]_{\sigma\sigma',\alpha\alpha'} \\
&= \sum_\tau \left[f^{\rm xcS}_{\sigma\sigma',\alpha\tau}(\mathbf{r},\mathbf{r}')n^*_{\tau\alpha'}(\mathbf{r}') + n^*_{\alpha\tau}(\mathbf{r}')f^{\rm xcS}_{\sigma\sigma',\tau\alpha'}(\mathbf{r},\mathbf{r}')\right],
\end{aligned}
$$

where we used $\underline{\underline{n}}^T = \underline{\underline{n}}^*$. This can be written in a 16-component block-diagonal matrix notation:

$$
\left(\begin{array}{cccccccccccccccc}
2n_{\uparrow\uparrow} & n^*_{\uparrow\downarrow} & n^*_{\downarrow\uparrow} & \\
n^*_{\downarrow\uparrow} & n & & n^*_{\downarrow\uparrow} \\
n^*_{\uparrow\downarrow} & & n & n^*_{\uparrow\downarrow} \\
& n^*_{\uparrow\downarrow} & n^*_{\downarrow\uparrow} & 2n_{\downarrow\downarrow} \\
&&&& 2n_{\uparrow\uparrow} & n^*_{\uparrow\downarrow} & n^*_{\downarrow\uparrow} & \\
&&&& n^*_{\downarrow\uparrow} & n & & n^*_{\downarrow\uparrow} \\
&&&& n^*_{\uparrow\downarrow} & & n & n^*_{\uparrow\downarrow} \\
&&&& & n^*_{\uparrow\downarrow} & n^*_{\downarrow\uparrow} & 2n_{\downarrow\downarrow} \\
&&&&&&&& 2n_{\uparrow\uparrow} & n^*_{\uparrow\downarrow} & n^*_{\downarrow\uparrow} & \\
&&&&&&&& n^*_{\downarrow\uparrow} & n & & n^*_{\downarrow\uparrow} \\
&&&&&&&& n^*_{\uparrow\downarrow} & & n & n^*_{\uparrow\downarrow} \\
&&&&&&&& & n^*_{\uparrow\downarrow} & n^*_{\downarrow\uparrow} & 2n_{\downarrow\downarrow} \\
&&&&&&&&&&&& 2n_{\uparrow\uparrow} & n^*_{\uparrow\downarrow} & n^*_{\downarrow\uparrow} & \\
&&&&&&&&&&&& n^*_{\downarrow\uparrow} & n & & n^*_{\downarrow\uparrow} \\
&&&&&&&&&&&& n^*_{\uparrow\downarrow} & & n & n^*_{\uparrow\downarrow} \\
&&&&&&&&&&&& & n^*_{\uparrow\downarrow} & n^*_{\downarrow\uparrow} & 2n_{\downarrow\downarrow}
\end{array}\right)
\left(\begin{array}{c}
f_{\uparrow\uparrow\uparrow\uparrow}\\ f_{\uparrow\uparrow\downarrow\uparrow}\\ f_{\uparrow\uparrow\uparrow\downarrow}\\ f_{\uparrow\uparrow\downarrow\downarrow}\\ f_{\downarrow\uparrow\uparrow\uparrow}\\ f_{\downarrow\uparrow\downarrow\uparrow}\\ f_{\downarrow\uparrow\uparrow\downarrow}\\ f_{\downarrow\uparrow\downarrow\downarrow}\\ f_{\uparrow\downarrow\uparrow\uparrow}\\ f_{\uparrow\downarrow\downarrow\uparrow}\\ f_{\uparrow\downarrow\uparrow\downarrow}\\ f_{\uparrow\downarrow\downarrow\downarrow}\\ f_{\downarrow\downarrow\uparrow\uparrow}\\ f_{\downarrow\downarrow\downarrow\uparrow}\\ f_{\downarrow\downarrow\uparrow\downarrow}\\ f_{\downarrow\downarrow\downarrow\downarrow}
\end{array}\right)
\qquad (31)
$$

We define the double vectorization operator $\mathbf{vec}^2$, which converts the $4\times 4$ matrix $f_{\sigma\sigma',\alpha\alpha'}$ into a column vector with 16 components:

$$
\mathbf{vec}^2\{\underline{\underline{f}}^{\rm xc}\} =
\left(\begin{array}{c}
f_{\uparrow\uparrow\uparrow\uparrow}\\ f_{\uparrow\uparrow\downarrow\uparrow}\\ f_{\uparrow\uparrow\uparrow\downarrow}\\ f_{\uparrow\uparrow\downarrow\downarrow}\\ f_{\downarrow\uparrow\uparrow\uparrow}\\ f_{\downarrow\uparrow\downarrow\uparrow}\\ f_{\downarrow\uparrow\uparrow\downarrow}\\ f_{\downarrow\uparrow\downarrow\downarrow}\\ f_{\uparrow\downarrow\uparrow\uparrow}\\ f_{\uparrow\downarrow\downarrow\uparrow}\\ f_{\uparrow\downarrow\uparrow\downarrow}\\ f_{\uparrow\downarrow\downarrow\downarrow}\\ f_{\downarrow\downarrow\uparrow\uparrow}\\ f_{\downarrow\downarrow\downarrow\uparrow}\\ f_{\downarrow\downarrow\uparrow\downarrow}\\ f_{\downarrow\downarrow\downarrow\downarrow}
\end{array}\right)
\qquad (32)
$$

Using $\underline{\underline{\mathcal{N}}}$ from Eq. (25), we can then write Eq. (31) as

$$
\begin{aligned}
&\left[\underline{\underline{f}}^{\rm xcS}\underline{\underline{n}}^*\right]_{\sigma\sigma',\alpha\alpha'} + \left[\underline{\underline{n}}^*\,\underline{\underline{f}}^{\rm xcS}\right]_{\sigma\sigma',\alpha\alpha'} \\
&= \left[\underline{\underline{I}}\otimes\underline{\underline{I}}\otimes\underline{\underline{\mathcal{N}}}^*(\mathbf{r}')\right]\mathbf{vec}^2\{\underline{\underline{f}}^{\rm xcS}(\mathbf{r},\mathbf{r}')\}.
\end{aligned}
\qquad (33)
$$

### 2. Approximating the functional derivatives

The second approximation is made in the evaluation of the functional derivatives $\delta v^{\rm xc}_{\sigma\sigma'}(\mathbf{r})/\delta\psi^*_{i\alpha'}(\mathbf{r}')$ and $\delta v^{\rm xc}_{\sigma\sigma'}(\mathbf{r})/\delta\psi_{i\alpha}(\mathbf{r}')$ in the right-hand side of Eq. (30). To simplify the functional derivatives, we only apply them to those parts in $v^{\rm xc}_{\sigma\sigma'}$ that are under an integral. Let us now explicitly work this out for the exchange-only case. We then have from Eq. (19)

$$
b_{\sigma\sigma'}(\mathbf{r}) = -2\sum_{kj}^N \psi_{j\sigma}(\mathbf{r})\psi^*_{k\sigma'}(\mathbf{r})\sum_\tau\int d\mathbf{r}'\,\frac{\psi^*_{j\tau}(\mathbf{r}')\psi_{k\tau}(\mathbf{r}')}{|\mathbf{r}-\mathbf{r}'|}
$$

so that we approximately get

$$\sum_i^N \left[ \frac{\delta b_{\sigma\sigma'}(\mathbf{r})}{\delta\psi^*_{i\alpha'}(\mathbf{r}')}\,\psi^*_{i\alpha}(\mathbf{r}') + \frac{\delta b_{\sigma\sigma'}(\mathbf{r})}{\delta\psi_{i\alpha}(\mathbf{r}')}\,\psi_{i\alpha'}(\mathbf{r}')\right]$$
$$\approx -2\sum_{ik}^N \psi_{i\sigma}(\mathbf{r})\psi^*_{k\sigma'}(\mathbf{r})\frac{1}{|\mathbf{r}-\mathbf{r}'|}\psi_{k\alpha'}(\mathbf{r}')\psi^*_{i\alpha}(\mathbf{r}')$$
$$-2\sum_{ij}^N \psi_{j\sigma}(\mathbf{r})\psi^*_{i\sigma'}(\mathbf{r})\frac{1}{|\mathbf{r}-\mathbf{r}'|}\psi^*_{j\alpha}(\mathbf{r}')\psi_{i\alpha'}(\mathbf{r}')$$
$$= -4\frac{\gamma_{\sigma\alpha}(\mathbf{r},\mathbf{r}')\gamma_{\alpha'\sigma'}(\mathbf{r}',\mathbf{r})}{|\mathbf{r}-\mathbf{r}'|}$$
$$\equiv d^{\mathrm{x}}_{\sigma\sigma',\alpha\alpha'}(\mathbf{r},\mathbf{r}')\,.$$

It is easy to see that this has the same symmetry properties as the xc kernel, see Eqs. (28) and (29):

$$d^{\mathrm{x}}_{\sigma'\sigma,\alpha'\alpha}(\mathbf{r},\mathbf{r}') = [d^{\mathrm{x}}_{\sigma\sigma',\alpha\alpha'}(\mathbf{r},\mathbf{r}')]^* \quad (34)$$
$$d^{\mathrm{x}}_{\alpha'\alpha,\sigma'\sigma}(\mathbf{r},\mathbf{r}') = d^{\mathrm{x}}_{\sigma\sigma',\alpha\alpha'}(\mathbf{r}',\mathbf{r})\,. \quad (35)$$

The right-hand side of Eq. (30) can then be written in a compact manner as

$$\mathbf{vec}^2\{\underline{\underline{R}}\} = \left[\underline{\underline{\mathcal{N}}}^{-1}(\mathbf{r})\otimes\underline{\underline{I}}\otimes\underline{\underline{I}}\right]\mathbf{vec}^2\{\underline{\underline{d}}^{\mathrm{x}}(\mathbf{r},\mathbf{r}')\}\,. \quad (36)$$

With this, Eq. (30) becomes:

$$\left[\underline{\underline{I}}\otimes\underline{\underline{I}}\otimes\underline{\underline{\mathcal{N}}}^{*}(\mathbf{r}')\right]\mathbf{vec}^2\{\underline{\underline{f}}^{\mathrm{xS}}(\mathbf{r},\mathbf{r}')\}$$
$$= \left[\underline{\underline{\mathcal{N}}}^{-1}(\mathbf{r})\otimes\underline{\underline{I}}\otimes\underline{\underline{I}}\right]\mathbf{vec}^2\{\underline{\underline{d}}^{\mathrm{x}}(\mathbf{r},\mathbf{r}')\}\,. \quad (37)$$

Let us define $\underline{\underline{I}}^4 = \underline{\underline{I}}\otimes\underline{\underline{I}}$, and we obtain

$$\mathbf{vec}^2\{\underline{\underline{f}}^{\mathrm{xS}}(\mathbf{r},\mathbf{r}')\}$$
$$= \left[\underline{\underline{I}}^4\otimes\underline{\underline{\mathcal{N}}}^{-1*}(\mathbf{r}')\right]\left[\underline{\underline{\mathcal{N}}}^{-1}(\mathbf{r})\otimes\underline{\underline{I}}^4\right]\mathbf{vec}^2\{\underline{\underline{d}}^{\mathrm{x}}(\mathbf{r},\mathbf{r}')\} \quad (38)$$

We use the Kronecker product rule $(A\otimes B)(C\otimes D) = (AC)\otimes(BD)$. The final result is

$$\mathbf{vec}^2\{\underline{\underline{f}}^{\mathrm{xS}}(\mathbf{r},\mathbf{r}')\} = \left[\underline{\underline{\mathcal{N}}}^{-1}(\mathbf{r})\otimes\underline{\underline{\mathcal{N}}}^{-1*}(\mathbf{r}')\right]\mathbf{vec}^2\{\underline{\underline{d}}^{\mathrm{x}}(\mathbf{r},\mathbf{r}')\}. \quad (39)$$

It can be proved that this satisfies the symmetry properties (28) and (29) of the xc kernel.

### C. Collinear limit

Let us now consider the case where the system has no transverse spin. In that case,

$$\underline{\underline{\mathcal{N}}}^{-1} = \frac{1}{2nn_{\uparrow\uparrow}n_{\downarrow\downarrow}}\begin{pmatrix} nn_{\downarrow\downarrow} & & & \\ & 2n_{\uparrow\uparrow}n_{\downarrow\downarrow} & & \\ & & 2n_{\uparrow\uparrow}n_{\downarrow\downarrow} & \\ & & & nn_{\uparrow\uparrow}\end{pmatrix}$$
$$= \frac{1}{2}\begin{pmatrix} n^{-1}_{\uparrow\uparrow} & & & \\ & 2n^{-1} & & \\ & & 2n^{-1} & \\ & & & n^{-1}_{\downarrow\downarrow}\end{pmatrix}$$

and

$$d^{\mathrm{x}}_{\sigma\sigma'\,\alpha\alpha'}(\mathbf{r},\mathbf{r}') = -4\frac{\gamma_{\sigma\alpha}(\mathbf{r},\mathbf{r}')\gamma_{\alpha'\sigma'}(\mathbf{r}',\mathbf{r})}{|\mathbf{r}-\mathbf{r}'|}\delta_{\sigma\alpha}\delta_{\sigma'\alpha'}\,.$$

Working out the exchange kernel is then straightforward, since $\underline{\underline{\mathcal{N}}}^{-1}(\mathbf{r})\otimes\underline{\underline{\mathcal{N}}}^{-1*}(\mathbf{r}')$ is diagonal. The only remaining terms are

$$\begin{pmatrix} f_{\uparrow\uparrow\uparrow\uparrow}\\ f_{\uparrow\downarrow\uparrow\downarrow}\\ f_{\downarrow\uparrow\downarrow\uparrow}\\ f_{\downarrow\downarrow\downarrow\downarrow}\end{pmatrix} = \begin{pmatrix} \underline{\underline{\mathcal{N}}}^{-1}_{11}(\mathbf{r})\underline{\underline{\mathcal{N}}}^{-1*}_{11}(\mathbf{r}')d^{\mathrm{x}}_{\uparrow\uparrow\uparrow\uparrow}\\ \underline{\underline{\mathcal{N}}}^{-1}_{22}(\mathbf{r})\underline{\underline{\mathcal{N}}}^{-1*}_{22}(\mathbf{r}')d^{\mathrm{x}}_{\uparrow\downarrow\uparrow\downarrow}\\ \underline{\underline{\mathcal{N}}}^{-1}_{33}(\mathbf{r})\underline{\underline{\mathcal{N}}}^{-1*}_{33}(\mathbf{r}')d^{\mathrm{x}}_{\downarrow\uparrow\downarrow\uparrow}\\ \underline{\underline{\mathcal{N}}}^{-1}_{44}(\mathbf{r})\underline{\underline{\mathcal{N}}}^{-1*}_{44}(\mathbf{r}')d^{\mathrm{x}}_{\downarrow\downarrow\downarrow\downarrow}\end{pmatrix}$$
$$= \frac{1}{4}\begin{pmatrix} \frac{1}{n_{\uparrow\uparrow}(\mathbf{r})n_{\uparrow\uparrow}(\mathbf{r}')}\,d^{\mathrm{x}}_{\uparrow\uparrow\uparrow\uparrow}\\ \frac{4}{n(\mathbf{r})n(\mathbf{r}')}\,d^{\mathrm{x}}_{\uparrow\downarrow\uparrow\downarrow}\\ \frac{4}{n(\mathbf{r})n(\mathbf{r}')}\,d^{\mathrm{x}}_{\downarrow\uparrow\downarrow\uparrow}\\ \frac{1}{n_{\downarrow\downarrow}(\mathbf{r})n_{\downarrow\downarrow}(\mathbf{r}')}\,d^{\mathrm{x}}_{\downarrow\downarrow\downarrow\downarrow}\end{pmatrix}$$

and the final results are

$$f^{\mathrm{xS}}_{\uparrow\uparrow\uparrow\uparrow}(\mathbf{r},\mathbf{r}') = -\frac{\gamma_{\uparrow\uparrow}(\mathbf{r},\mathbf{r}')\gamma_{\uparrow\uparrow}(\mathbf{r}',\mathbf{r})}{n_{\uparrow\uparrow}(\mathbf{r})n_{\uparrow\uparrow}(\mathbf{r}')|\mathbf{r}-\mathbf{r}'|} \quad (40)$$
$$f^{\mathrm{xS}}_{\downarrow\downarrow\downarrow\downarrow}(\mathbf{r},\mathbf{r}') = -\frac{\gamma_{\downarrow\downarrow}(\mathbf{r},\mathbf{r}')\gamma_{\downarrow\downarrow}(\mathbf{r}',\mathbf{r})}{n_{\downarrow\downarrow}(\mathbf{r})n_{\downarrow\downarrow}(\mathbf{r}')|\mathbf{r}-\mathbf{r}'|} \quad (41)$$
$$f^{\mathrm{xS}}_{\uparrow\downarrow\uparrow\downarrow}(\mathbf{r},\mathbf{r}') = -4\frac{\gamma_{\uparrow\uparrow}(\mathbf{r},\mathbf{r}')\gamma_{\downarrow\downarrow}(\mathbf{r}',\mathbf{r})}{n(\mathbf{r})n(\mathbf{r}')|\mathbf{r}-\mathbf{r}'|} \quad (42)$$
$$f^{\mathrm{xS}}_{\downarrow\uparrow\downarrow\uparrow}(\mathbf{r},\mathbf{r}') = -4\frac{\gamma_{\downarrow\downarrow}(\mathbf{r},\mathbf{r}')\gamma_{\uparrow\uparrow}(\mathbf{r}',\mathbf{r})}{n(\mathbf{r})n(\mathbf{r}')|\mathbf{r}-\mathbf{r}'|}\,, \quad (43)$$

see Eqs. (35), (36) in the main paper. $f^{\mathrm{xS}}_{\uparrow\uparrow\uparrow\uparrow}$ and $f^{\mathrm{xS}}_{\downarrow\downarrow\downarrow\downarrow}$ are the PGG exchange kernels,[2,3] $f^{\mathrm{xS}}_{\uparrow\downarrow\uparrow\downarrow}$ and $f^{\mathrm{xS}}_{\downarrow\uparrow\downarrow\uparrow}$ are new.

### D. Reconstruction of the Slater potential

Now we need to reconstruct the Slater exchange potential from the PGG exchange kernel. First of all, we compare

$$d^{\mathrm{x}}_{\sigma\sigma',\alpha\alpha'}(\mathbf{r},\mathbf{r}') = -4\frac{\gamma_{\sigma\alpha}(\mathbf{r},\mathbf{r}')\gamma_{\alpha'\sigma'}(\mathbf{r}',\mathbf{r})}{|\mathbf{r}-\mathbf{r}'|}$$

with

$$b_{\sigma\sigma'} = -2\sum_\tau\int\frac{d\mathbf{r}'}{|\mathbf{r}-\mathbf{r}'|}\gamma_{\sigma\tau}(\mathbf{r},\mathbf{r}')\gamma_{\tau\sigma'}(\mathbf{r}',\mathbf{r})$$

and we see from this that

$$b_{\sigma\sigma'} = \frac{1}{2}\sum_\tau\int d\mathbf{r}'\,d^{\mathrm{x}}_{\sigma\sigma',\tau\tau}(\mathbf{r},\mathbf{r}')\,. \quad (44)$$

We can now express Eq. (44) in matrix-vector form as

$$\begin{pmatrix} b_{\uparrow\uparrow}(\mathbf{r}) \\ 0 \\ 0 \\ 0 \\ b_{\downarrow\uparrow}(\mathbf{r}) \\ 0 \\ 0 \\ 0 \\ b_{\uparrow\downarrow}(\mathbf{r}) \\ 0 \\ 0 \\ 0 \\ b_{\downarrow\downarrow}(\mathbf{r}) \\ 0 \\ 0 \\ 0 \end{pmatrix} = \frac{1}{2}\int d\mathbf{r}' \begin{pmatrix} 1 &&& 1 &&&&&&&&&&&& \\ &&&&&&&&&&&&&&& \\ &&&&&&&&&&&&&&& \\ &&&&&&&&&&&&&&& \\ &&&& 1 &&& 1 &&&&&&&& \\ &&&&&&&&&&&&&&& \\ &&&&&&&&&&&&&&& \\ &&&&&&&&&&&&&&& \\ &&&&&&&& 1 &&& 1 &&&& \\ &&&&&&&&&&&&&&& \\ &&&&&&&&&&&&&&& \\ &&&&&&&&&&&&&&& \\ &&&&&&&&&&&& 1 &&& 1 \\ &&&&&&&&&&&&&&& \\ &&&&&&&&&&&&&&& \\ &&&&&&&&&&&&&&& \end{pmatrix} \begin{pmatrix} d^{\mathrm{x}}_{\uparrow\uparrow\uparrow\uparrow} \\ d^{\mathrm{x}}_{\uparrow\uparrow\downarrow\uparrow} \\ d^{\mathrm{x}}_{\uparrow\uparrow\uparrow\downarrow} \\ d^{\mathrm{x}}_{\uparrow\uparrow\downarrow\downarrow} \\ d^{\mathrm{x}}_{\downarrow\uparrow\uparrow\uparrow} \\ d^{\mathrm{x}}_{\downarrow\uparrow\downarrow\uparrow} \\ d^{\mathrm{x}}_{\downarrow\uparrow\uparrow\downarrow} \\ d^{\mathrm{x}}_{\downarrow\uparrow\downarrow\downarrow} \\ d^{\mathrm{x}}_{\uparrow\downarrow\uparrow\uparrow} \\ d^{\mathrm{x}}_{\uparrow\downarrow\downarrow\uparrow} \\ d^{\mathrm{x}}_{\uparrow\downarrow\uparrow\downarrow} \\ d^{\mathrm{x}}_{\uparrow\downarrow\downarrow\downarrow} \\ d^{\mathrm{x}}_{\downarrow\downarrow\uparrow\uparrow} \\ d^{\mathrm{x}}_{\downarrow\downarrow\downarrow\uparrow} \\ d^{\mathrm{x}}_{\downarrow\downarrow\uparrow\downarrow} \\ d^{\mathrm{x}}_{\downarrow\downarrow\downarrow\downarrow} \end{pmatrix}$$

or, more compactly,

$$\mathbf{vec}\{\underline{\underline{b}}\} \otimes \mathbf{vec}\{\underline{\underline{m}}\} = \frac{1}{2}\int d\mathbf{r}' \left[\underline{\underline{I}}^4 \otimes \underline{\underline{T}}\right] \mathbf{vec}^2\{\underline{\underline{d}}^{\mathrm{x}}(\mathbf{r},\mathbf{r}')\}, \tag{45}$$

where

$$\underline{\underline{m}} = \begin{pmatrix} 1 & 0 \\ 0 & 0 \end{pmatrix} \qquad \underline{\underline{T}} = \begin{pmatrix} 1 & 0 & 0 & 1 \\ 0 & 0 & 0 & 0 \\ 0 & 0 & 0 & 0 \\ 0 & 0 & 0 & 0 \end{pmatrix}.$$

Now let's express this through the exchange kernel. From Eq. (39) it follows, using the Kronecker product rule, that

$$\mathbf{vec}^2\{\underline{\underline{d}}^{\mathrm{x}}(\mathbf{r},\mathbf{r}')\} = \left[\underline{\underline{\mathcal{N}}}(\mathbf{r}) \otimes \underline{\underline{\mathcal{N}}}^*(\mathbf{r}')\right] \mathbf{vec}^2\{\underline{\underline{f}}^{\mathrm{xS}}(\mathbf{r},\mathbf{r}')\} \tag{46}$$

and substituting this into Eq. (45) we get

$$\begin{aligned} \mathbf{vec}\{\underline{\underline{b}}\} \otimes \mathbf{vec}\{\underline{\underline{m}}\} &= \frac{1}{2}\int d\mathbf{r}' \left[\underline{\underline{I}}^4 \otimes \underline{\underline{T}}\right] \left[\underline{\underline{\mathcal{N}}}(\mathbf{r}) \otimes \underline{\underline{\mathcal{N}}}^*(\mathbf{r}')\right] \mathbf{vec}^2\{\underline{\underline{f}}^{\mathrm{xS}}(\mathbf{r},\mathbf{r}')\} \\ &= \frac{1}{2}\int d\mathbf{r}' \left[\underline{\underline{\mathcal{N}}}(\mathbf{r}) \otimes \underline{\underline{T}}\,\underline{\underline{\mathcal{N}}}^*(\mathbf{r}')\right] \mathbf{vec}^2\{\underline{\underline{f}}^{\mathrm{xS}}(\mathbf{r},\mathbf{r}')\}\,. \end{aligned} \tag{47}$$

Finally, let us construct the Slater potential from this. We can write Eq. (26) as

$$\mathbf{vec}\left\{\underline{\underline{v}}^{\mathrm{xS}}(\mathbf{r})\right\} \otimes \mathbf{vec}\{\underline{\underline{m}}\} = \left[\underline{\underline{\mathcal{N}}}^{-1}(\mathbf{r}) \otimes \underline{\underline{S}}\right] \left[\mathbf{vec}\{\underline{\underline{b}}(\mathbf{r})\} \otimes \mathbf{vec}\{\underline{\underline{m}}\}\right], \tag{48}$$

where

$$\underline{\underline{S}} = \begin{pmatrix} 1 & 0 & 0 & 0 \\ 0 & 0 & 0 & 0 \\ 0 & 0 & 0 & 0 \\ 0 & 0 & 0 & 0 \end{pmatrix}$$

and hence

$$\begin{aligned} \mathbf{vec}\left\{\underline{\underline{v}}^{\mathrm{xS}}(\mathbf{r})\right\} \otimes \mathbf{vec}\{\underline{\underline{m}}\} &= \frac{1}{2}\int d\mathbf{r}' \left[\underline{\underline{\mathcal{N}}}^{-1}(\mathbf{r}) \otimes \underline{\underline{S}}\right] \left[\underline{\underline{\mathcal{N}}}(\mathbf{r}) \otimes \underline{\underline{T}}\,\underline{\underline{\mathcal{N}}}^*(\mathbf{r}')\right] \mathbf{vec}^2\{\underline{\underline{f}}^{\mathrm{xS}}(\mathbf{r},\mathbf{r}')\} \\ &= \frac{1}{2}\int d\mathbf{r}' \left[\underline{\underline{I}}^4 \otimes \underline{\underline{T}}\,\underline{\underline{\mathcal{N}}}^*(\mathbf{r}')\right] \mathbf{vec}^2\{\underline{\underline{f}}^{\mathrm{xS}}(\mathbf{r},\mathbf{r}')\}. \end{aligned} \tag{49}$$

We have

$$\underline{\underline{T}}\,\underline{\underline{\mathcal{N}}}^{*} = 2\begin{pmatrix} n_{\uparrow\uparrow} & n_{\downarrow\uparrow} & n_{\uparrow\downarrow} & n_{\downarrow\downarrow} \\ 0 & 0 & 0 & 0 \\ 0 & 0 & 0 & 0 \\ 0 & 0 & 0 & 0 \end{pmatrix}$$

or in detail

$$\begin{pmatrix} v^{\rm xS}_{\uparrow\uparrow} \\ 0 \\ 0 \\ 0 \\ v^{\rm xS}_{\downarrow\uparrow} \\ 0 \\ 0 \\ 0 \\ v^{\rm xS}_{\uparrow\downarrow} \\ 0 \\ 0 \\ 0 \\ v^{\rm xS}_{\downarrow\downarrow} \\ 0 \\ 0 \\ 0 \end{pmatrix} = \int d\mathbf{r}' \left(\begin{array}{cccccccccccccccc} n_{\uparrow\uparrow} & n_{\downarrow\uparrow} & n_{\uparrow\downarrow} & n_{\downarrow\downarrow} & & & & & & & & & & & & \\ & & & & & & & & & & & & & & & \\ & & & & & & & & & & & & & & & \\ & & & & & & & & & & & & & & & \\ & & & & n_{\uparrow\uparrow} & n_{\downarrow\uparrow} & n_{\uparrow\downarrow} & n_{\downarrow\downarrow} & & & & & & & & \\ & & & & & & & & & & & & & & & \\ & & & & & & & & & & & & & & & \\ & & & & & & & & & & & & & & & \\ & & & & & & & & n_{\uparrow\uparrow} & n_{\downarrow\uparrow} & n_{\uparrow\downarrow} & n_{\downarrow\downarrow} & & & & \\ & & & & & & & & & & & & & & & \\ & & & & & & & & & & & & & & & \\ & & & & & & & & & & & & & & & \\ & & & & & & & & & & & & n_{\uparrow\uparrow} & n_{\downarrow\uparrow} & n_{\uparrow\downarrow} & n_{\downarrow\downarrow} \\ & & & & & & & & & & & & & & & \\ & & & & & & & & & & & & & & & \\ & & & & & & & & & & & & & & & \end{array}\right) \begin{pmatrix} f^{\rm xS}_{\uparrow\uparrow\uparrow\uparrow} \\ f^{\rm xS}_{\uparrow\uparrow\downarrow\uparrow} \\ f^{\rm xS}_{\uparrow\uparrow\uparrow\downarrow} \\ f^{\rm xS}_{\uparrow\uparrow\downarrow\downarrow} \\ f^{\rm xS}_{\downarrow\uparrow\uparrow\uparrow} \\ f^{\rm xS}_{\downarrow\uparrow\downarrow\uparrow} \\ f^{\rm xS}_{\downarrow\uparrow\uparrow\downarrow} \\ f^{\rm xS}_{\downarrow\uparrow\downarrow\downarrow} \\ f^{\rm xS}_{\uparrow\downarrow\uparrow\uparrow} \\ f^{\rm xS}_{\uparrow\downarrow\downarrow\uparrow} \\ f^{\rm xS}_{\uparrow\downarrow\uparrow\downarrow} \\ f^{\rm xS}_{\uparrow\downarrow\downarrow\downarrow} \\ f^{\rm xS}_{\downarrow\downarrow\uparrow\uparrow} \\ f^{\rm xS}_{\downarrow\downarrow\downarrow\uparrow} \\ f^{\rm xS}_{\downarrow\downarrow\uparrow\downarrow} \\ f^{\rm xS}_{\downarrow\downarrow\downarrow\downarrow} \end{pmatrix}$$

so it is immediately clear that

$$v^{\rm Slater}_{\sigma\sigma'}(\mathbf{r}) = \sum_{\tau\tau'} \int d\mathbf{r}' f^{\rm xS}_{\sigma\sigma',\tau\tau'}(\mathbf{r},\mathbf{r}') n_{\tau\tau'}(\mathbf{r}') \,. \tag{50}$$

Alternatively, we can express this as

$$v^{\rm Slater}_{\sigma\sigma'}(\mathbf{r}) = \frac{1}{2}\sum_{\beta\beta'\tau} \int d\mathbf{r}' \mathcal{N}^{-1}_{\sigma\sigma',\beta\beta'}(\mathbf{r}) d_{\beta\beta',\tau\tau}(\mathbf{r},\mathbf{r}') \,, \tag{51}$$

which is consistent with Eqs. (26) and (44).

## III. SPECTRAL REPRESENTATION OF THE RESPONSE FUNCTION

The Casida equation is used in linear-response TDDFT to calculate excitation energies. One assumes that there is no external perturbation and calculates the electronic eigenmodes of the system. For noncollinear spin systems, the Casida equation reads as follows:[4,5]

$$\sum_{i'a'} \left\{ \Big[\delta_{ii'}\delta_{aa'}\omega_{a'i'} + K_{ia,i'a'}\Big] X^{(m)}_{i'a'} + K_{ia,a'i'} Y^{(m)}_{i'a'} \right\} = -\Omega_m X^{(m)}_{ia} \tag{52}$$

$$\sum_{i'a'} \left\{ K_{ai,i'a'} X^{(m)}_{i'a'} + \Big[\delta_{aa'}\delta_{ii'}\omega_{a'i'} + K_{ai,a'i'}\Big] Y^{(m)}_{i'a'} \right\} = \Omega_m Y^{(m)}_{ia} \,, \tag{53}$$

where $i, i'$ and $a, a'$ run over occupied and unoccupied orbitals, respectively, and $\omega_{ai} = \epsilon_a - \epsilon_i$ are the Kohn-Sham excitation energies. The coupling matrix elements are defined as

$$K_{pq,p'q'} = \sum_{\alpha\alpha'}\sum_{\sigma\sigma'} \int d\mathbf{x} \int d\mathbf{r} \Phi_{p'\alpha q'\alpha'}(\mathbf{x}) \times f^{\rm Hxc}_{\alpha\alpha',\sigma\sigma'}(\mathbf{x},\mathbf{r}) \Phi^{*}_{p\sigma q\sigma'}(\mathbf{r}) \,, \tag{54}$$

where $\Phi_{p\sigma q\sigma'}(\mathbf{r}) = \psi^{*}_{p\sigma}(\mathbf{r})\psi_{q\sigma'}(\mathbf{r})$, and $p, q, p', q'$ are the orbital indices referred to in Eqs. (52) and (53). Solving the Casida equation gives the excitation energies $\Omega_m$.

Let us now consider the case where there is a frequency-dependent perturbing potential $v_{\tau\tau'}(\mathbf{r},\omega)$. One can then recast the TDDFT linear response equation into a form that is analogous to the Casida equations (52) and (53):

$$\sum_{i'a'} \left\{ \Big[\delta_{ii'}\delta_{aa'}\omega_{a'i'} + K_{ia,i'a'}\Big] X_{i'a'} + K_{ia,a'i'} Y_{i'a'} \right\} + \omega X_{ia} = -v_{ia}(\omega) \tag{55}$$

$$\sum_{i'a'} \left\{ K_{ai,i'a'} X_{i'a'} + \Big[\delta_{aa'}\delta_{ii'}\omega_{a'i'} + K_{ai,a'i'}\Big] Y_{i'a'} \right\} - \omega Y_{ia} = -v_{ai}(\omega) \,, \tag{56}$$

where the matrix elements of the perturbing potential are given by

$$v_{pq}(\omega) = \sum_{\tau\tau'} \int d\mathbf{r}' \, \Phi_{p\tau q\tau'}(\mathbf{r}') v_{\tau\tau'}(\mathbf{r}',\omega) \,. \tag{57}$$

The density response to the given perturbation is then obtained from the solutions of Eqs. (55) and (56):

$$\delta n_{\sigma\sigma'}(\mathbf{r},\omega) = \sum_{ia} \left[\Phi^*_{i\sigma a\sigma'}(\mathbf{r}) X_{ia}(\omega) + \Phi_{i\sigma' a\sigma}(\mathbf{r}) Y_{ia}(\omega)\right] . \tag{58}$$

Now consider a special form of the perturbation:

$$v_{\tau\tau'}(\mathbf{r},\omega) = \delta_{\tau\gamma}\delta_{\tau'\gamma'}\delta(\mathbf{r}-\mathbf{y}) , \tag{59}$$

where $\mathbf{y}$ is an arbitrary reference point. The linear density response is then equal to the response function itself:

$$\begin{aligned}\delta n_{\sigma\sigma'}(\mathbf{r},\omega) &= \sum_{\tau\tau'} \int d^3r' \chi_{\sigma\sigma',\tau\tau'}(\mathbf{r},\mathbf{r}',\omega) v_{\tau\tau'}(\mathbf{r}',\omega) \\ &= \chi_{\sigma\sigma',\gamma\gamma'}(\mathbf{r},\mathbf{y},\omega) . \end{aligned} \tag{60}$$

For the special perturbation (59), we have from Eq. (57)

$$v_{jk}(\omega) = \Phi_{j\gamma k\gamma'}(\mathbf{y}) . \tag{61}$$

If we use this as the right-hand side of Eqs. (55) and (56), the solution vectors $X_{ia}$ and $Y_{ia}$ will depend parametrically on $\gamma, \gamma'$ and $\mathbf{y}$: $X_{ia}^{\gamma\gamma'}(\mathbf{y})$ and $Y_{ia}^{\gamma\gamma'}(\mathbf{y})$. Comparing Eqs. (58) and (60), we obtain the following expression for the response function:

$$\begin{aligned}\chi_{\sigma\sigma',\gamma\gamma'}(\mathbf{r},\mathbf{y},\omega) = \sum_{ia} \Big[&\Phi^*_{i\sigma a\sigma'}(\mathbf{r}) X_{ia}^{\gamma\gamma'}(\mathbf{y},\omega) \\ &+ \Phi_{i\sigma' a\sigma}(\mathbf{r}) Y_{ia}^{\gamma\gamma'}(\mathbf{y},\omega)\Big] . \end{aligned} \tag{62}$$

We would like to have the form of a Lehmann representation, where the poles at the exact excitation energies show up explicitly. To this end, we use the spectral expansion of the solutions $X_{ia}$ and $Y_{ia}$, written in vector form,[6] in terms of the eigenvectors of the Casida equation, $X_{ia}^{(m)}$ and $Y_{ia}^{(m)}$:

$$|\mathbf{X},\mathbf{Y}\rangle = \sum_m \mathrm{sign}(\Omega_m) \frac{|\mathbf{X}_m,\mathbf{Y}_m\rangle\langle -\mathbf{X}_m,\mathbf{Y}_m|\mathbf{v},-\mathbf{v}^\dagger\rangle}{\Omega_m - \omega} , \tag{63}$$

which gives

$$\begin{pmatrix} \mathbf{X} \\ \mathbf{Y} \end{pmatrix} = \sum_m \mathrm{sign}(\Omega_m) \begin{pmatrix} \mathbf{X}_m \\ \mathbf{Y}_m \end{pmatrix} \frac{\langle \mathbf{X}_m|\mathbf{v}\rangle + \langle \mathbf{Y}_m|\mathbf{v}^\dagger\rangle}{\omega - \Omega_m} , \tag{64}$$

where the vectors $\mathbf{v}$ and $\mathbf{v}^\dagger$ have the components

$$\begin{aligned}\mathbf{v} &\to v_{ia} = \Phi_{i\gamma a\gamma'}(\mathbf{y}) \\ \mathbf{v}^\dagger &\to v_{ai} = \Phi_{a\gamma i\gamma'}(\mathbf{y}) = \Phi^*_{i\gamma' a\gamma}(\mathbf{y}) . \end{aligned}$$

Substituting this into Eq. (62) gives the expression for the response function used in the main paper, see Eq. (45) there.

## IV. STLS EXCHANGE-CORRELATION ENERGY

The total ground-state energy is given by

$$\begin{aligned} E_0 = &\sum_j^N \epsilon_j - \frac{1}{2}\int d\mathbf{r} \int d\mathbf{r}' \frac{n(\mathbf{r})n(\mathbf{r}')}{|\mathbf{r}-\mathbf{r}'|} + E_{\mathrm{xc}}[\underline{\underline{n}}] \\ &- \sum_{\sigma\sigma'} \int d\mathbf{r}\, n_{\sigma\sigma'}(r) v^{\mathrm{xc}}_{\sigma'\sigma}(r) . \end{aligned} \tag{65}$$

In STLS, we have an approximate expression for the xc potential, but we do not know the functional $E_{\mathrm{xc}}[\underline{\underline{n}}]$ a priori. To obtain it, we will need a coupling constant integration.

It is well known that the exchange energy can be expressed in terms of the exchange hole density $n_{\mathrm{x}}(\mathbf{r},\mathbf{r}')$:

$$E_{\mathrm{x}} = \frac{1}{2}\int d\mathbf{r} \int d\mathbf{r}' \frac{n(\mathbf{r})n_{\mathrm{x}}(\mathbf{r},\mathbf{r}')}{|\mathbf{r}-\mathbf{r}'|} . \tag{66}$$

Similarly, the xc energy is given by

$$E_{\mathrm{xc}} = \frac{1}{2}\int d\mathbf{r} \int d\mathbf{r}' \frac{n(\mathbf{r})\bar{n}_{\mathrm{xc}}(\mathbf{r},\mathbf{r}')}{|\mathbf{r}-\mathbf{r}'|} , \tag{67}$$

where

$$\bar{n}_{\mathrm{xc}}(\mathbf{r},\mathbf{r}') = \int_0^1 d\lambda\, n^\lambda_{\mathrm{xc}}(\mathbf{r},\mathbf{r}') \tag{68}$$

is the coupling constant averaged xc hole. We need to express the xc hole in terms of the static structure factor, since that is the object that is calculated in STLS.

We start with the electron-electron interaction energy:[7]

$$W = \frac{1}{2}\sum_{\alpha\beta} \int d\mathbf{r} \int d\mathbf{r}' \frac{\rho^{(2)}_{\alpha\beta}(\mathbf{r},\mathbf{r}')}{|\mathbf{r}-\mathbf{r}'|} , \tag{69}$$

which involves the two-particle spin density matrix. Notice that there are only two spin indices; more precisely, we have $\rho^{(2)}_{\alpha\beta}(\mathbf{r},\mathbf{r}') = \gamma_{\alpha\alpha,\beta\beta}(\mathbf{r},\mathbf{r}';\mathbf{r},\mathbf{r}')$, where the two-particle density matrix is defined in second quantization (using Fermionic field operators) as

$$\gamma_{\alpha\alpha',\beta\beta'}(\mathbf{r},\mathbf{r}';\mathbf{r},\mathbf{r}') = \langle \hat\psi^\dagger_{\alpha'}(\mathbf{r})\hat\psi^\dagger_{\beta'}(\mathbf{r}')\hat\psi_\beta(\mathbf{r}')\hat\psi_\alpha(\mathbf{r})\rangle. \tag{70}$$

There is a connection between the two-particle density matrix and the pair correlation function $g$:

$$g_{\gamma\alpha',\beta\delta}(\mathbf{r},\mathbf{r}') = \sum_{\alpha\beta'} n^{-1}_{\gamma\alpha}(\mathbf{r})\gamma_{\alpha\alpha',\beta\beta'}(\mathbf{r},\mathbf{r}') n^{-1}_{\beta'\delta}(\mathbf{r}') ,$$

which can be inverted as

$$\gamma_{\alpha\alpha',\beta\beta'}(\mathbf{r},\mathbf{r}') = \sum_{\gamma\delta} n_{\alpha\gamma}(\mathbf{r}) g_{\gamma\alpha',\beta\delta}(\mathbf{r},\mathbf{r}') n_{\delta\beta'}(\mathbf{r}') .$$

Therefore,

$$\rho^{(2)}_{\alpha\beta}(\mathbf{r},\mathbf{r}') = \sum_{\gamma\delta} n_{\alpha\gamma}(\mathbf{r}) g_{\gamma\alpha,\beta\delta}(\mathbf{r},\mathbf{r}') n_{\delta\beta}(\mathbf{r}') \,. \tag{71}$$

Substituting this into Eq. (69) gives

$$W = \frac{1}{2}\sum_{\alpha\beta}\sum_{\gamma\delta}\int d\mathbf{r}\int d\mathbf{r}' \, \frac{n_{\alpha\gamma}(\mathbf{r}) g_{\gamma\alpha,\beta\delta}(\mathbf{r},\mathbf{r}') n_{\delta\beta}(\mathbf{r}')}{|\mathbf{r}-\mathbf{r}'|} \,. \tag{72}$$

Now let us express this in terms of the spin-resolved static structure factor. We derive the connection using the noninteracting case, where the pair correlation function is

$$\begin{aligned} g^0_{\alpha\alpha',\beta\beta'}(\mathbf{r},\mathbf{r}') = {}& \delta_{\alpha\alpha'}\delta_{\beta\beta'} \\ & - \sum_{\tau\tau'} n^{-1}_{\alpha\tau}(\mathbf{r}) \gamma_{\beta\alpha'}(\mathbf{r}',\mathbf{r}) \gamma_{\tau\tau'}(\mathbf{r},\mathbf{r}') n^{-1}_{\tau',\beta'}(\mathbf{r}') \end{aligned} \tag{73}$$

so that the product of one-particle density matrices, see Eq. (16), is given by

$$\begin{aligned} \gamma_{\sigma\sigma'}(\mathbf{r},\mathbf{r}')\gamma_{\beta\alpha}(\mathbf{r}',\mathbf{r}) = {}& n_{\sigma\alpha}(\mathbf{r}) n_{\beta\sigma'}(\mathbf{r}') \\ & - \sum_{\alpha'\beta'} n_{\sigma\alpha'}(\mathbf{r}) g^0_{\alpha'\alpha,\beta\beta'}(\mathbf{r},\mathbf{r}') n_{\beta'\sigma'}(\mathbf{r}'). \end{aligned} \tag{74}$$

Now compare this to the noninteracting structure factor

$$S^0_{\sigma\sigma',\tau\tau'}(\mathbf{r},\mathbf{r}') = \delta_{\sigma\tau}\delta(\mathbf{r}-\mathbf{r}') n_{\tau'\sigma'}(\mathbf{r}) - \gamma_{\sigma\tau}(\mathbf{r},\mathbf{r}')\gamma_{\tau'\sigma'}(\mathbf{r}',\mathbf{r}), \tag{75}$$

and we find, renaming $\sigma' \to \tau$ and $\beta \to \tau'$ and $\alpha \to \sigma'$,

$$\begin{aligned} \gamma_{\sigma\tau}(\mathbf{r},\mathbf{r}')\gamma_{\tau'\sigma'}(\mathbf{r}',\mathbf{r}) = {}& n_{\sigma\sigma'}(\mathbf{r}) n_{\tau'\tau}(\mathbf{r}') \\ & - \sum_{\alpha'\beta'} n_{\sigma\alpha'}(\mathbf{r}) g^0_{\alpha'\sigma',\tau'\beta'}(\mathbf{r},\mathbf{r}') n_{\beta'\tau}(\mathbf{r}') \end{aligned} \tag{76}$$

and hence

$$\begin{aligned} S^0_{\sigma\sigma',\tau\tau'}(\mathbf{r},\mathbf{r}') = {}& \delta_{\sigma\tau}\delta(\mathbf{r}-\mathbf{r}') n_{\tau'\sigma'}(\mathbf{r}) - n_{\sigma\sigma'}(\mathbf{r}) n_{\tau'\tau}(\mathbf{r}') \\ & + \sum_{\alpha'\beta'} n_{\sigma\alpha'}(\mathbf{r}) g^0_{\alpha'\sigma',\tau'\beta'}(\mathbf{r},\mathbf{r}') n_{\beta'\tau}(\mathbf{r}'). \end{aligned} \tag{77}$$

This relation between the structure factor and the pair correlation function will remain valid in the interacting case. In expression (72) for the interaction energy, we need $S_{\alpha\alpha,\beta\beta}$, which is given by

$$\begin{aligned} S_{\alpha\alpha,\beta\beta}(\mathbf{r},\mathbf{r}') = {}& \delta_{\alpha\beta}\delta(\mathbf{r}-\mathbf{r}') n_{\beta\alpha}(\mathbf{r}) - n_{\alpha\alpha}(\mathbf{r}) n_{\beta\beta}(\mathbf{r}') \\ & + \sum_{\gamma\delta} n_{\alpha\gamma}(\mathbf{r}) g_{\gamma\alpha,\beta\delta}(\mathbf{r},\mathbf{r}') n_{\delta\beta}(\mathbf{r}') \end{aligned} \tag{78}$$

and thus

$$\begin{aligned} W &= \frac{1}{2}\sum_{\alpha\beta}\int d\mathbf{r}\int d\mathbf{r}' \, \frac{1}{|\mathbf{r}-\mathbf{r}'|}\left[S_{\alpha\alpha,\beta\beta}(\mathbf{r},\mathbf{r}') - \delta_{\alpha\beta}\delta(\mathbf{r}-\mathbf{r}') n_{\beta\alpha}(\mathbf{r}) + n_{\alpha\alpha}(\mathbf{r}) n_{\beta\beta}(\mathbf{r}')\right] \\ &= \frac{1}{2}\sum_{\alpha\beta}\int d\mathbf{r}\int d\mathbf{r}' \, \frac{S_{\alpha\alpha,\beta\beta}(\mathbf{r},\mathbf{r}') - \delta(\mathbf{r}-\mathbf{r}') n(\mathbf{r})}{|\mathbf{r}-\mathbf{r}'|} + \frac{1}{2}\int d\mathbf{r}\int d\mathbf{r}' \, \frac{n(\mathbf{r}) n(\mathbf{r}')}{|\mathbf{r}-\mathbf{r}'|} \,. \end{aligned} \tag{79}$$

The xc energy is given by

$$E_{\rm xc} = \int_0^1 d\lambda W_\lambda - E_{\rm H}, \tag{80}$$

where the Hartree energy $E_{\rm H}$ is the last term on the right-hand side of Eq. (79). $W_\lambda$ is the full electron-electron interaction energy using the many-body ground-state of the system scaled by $\lambda$. We thus end up with

$$E_{\rm xc} = \frac{1}{2}\int d\mathbf{r}\int d\mathbf{r}' \, \frac{\sum_{\alpha\beta}\bar{S}_{\alpha\alpha,\beta\beta}(\mathbf{r},\mathbf{r}') - \delta(\mathbf{r}-\mathbf{r}') n(\mathbf{r})}{|\mathbf{r}-\mathbf{r}'|} \,, \tag{81}$$

where $\bar{S}$ denotes the coupling constant average.

In Eq. (38) in the main paper we had established

$$\begin{aligned} d^{\rm xc}_{\alpha\alpha,\beta\beta}(\mathbf{r},\mathbf{r}') = {}& \frac{4}{|\mathbf{r}-\mathbf{r}'|}\Big[S_{\alpha\alpha,\beta\beta}(\mathbf{r},\mathbf{r}') \\ & - \delta_{\alpha\beta}\delta(\mathbf{r}-\mathbf{r}') n_{\beta\alpha}(\mathbf{r})\Big], \end{aligned} \tag{82}$$

where

$$\mathbf{vec}^2\{\underline{\underline{d}}^{\rm xc}(\mathbf{r},\mathbf{r}')\} = \left[\underline{\underline{\mathcal{N}}}(\mathbf{r}) \otimes \underline{\underline{\mathcal{N}}}^*(\mathbf{r}')\right] \mathbf{vec}\{\underline{\underline{f}}^{\rm xc}(\mathbf{r},\mathbf{r}')\} \,. \tag{83}$$

So the xc energy becomes

$$E_{\rm xc} = \frac{1}{8}\sum_{\alpha\beta}\int d\mathbf{r}\int d\mathbf{r}' \, \bar{d}_{\alpha\alpha,\beta\beta}(\mathbf{r},\mathbf{r}') \,. \tag{84}$$

The problem of calculating the xc energy is thus reduced to calculating the coupling-constant averaged xc kernel.

We define $f^{\rm xc,\lambda}_{\alpha\beta,\gamma\delta}$ as that xc kernel which follows from the STLS scheme by using $\lambda f_{\rm Hxc}$ to solve the Casida equation [in other words, we include a factor $\lambda$ in the $K$-matrix in Eqs. (52) and (53)], which then gives the spectral representation of the static structure factor $S^\lambda$, see Eq. (46) of the main text.

[1] J. B. Krieger, Y. Li, and G. J. Iafrate, Phys. Rev. A **45**, 101 (1992).
[2] M. Petersilka, U. J. Gossmann, and E. K. U. Gross, Phys. Rev. Lett. **76**, 1212 (1996).
[3] M. Petersilka, U. J. Gossmann, and E. K. U. Gross, in *Electronic density functional theory: recent progress and new directions*, edited by J. F. Dobson, G. Vignale, and M. P. Das (Plenum, New York, 1998) pp. 177–97.
[4] C. A. Ullrich, *Time-dependent density-functional theory: concepts and applications* (Oxford University Press, Oxford, 2012).
[5] M. E. Casida, in *Recent Advances in Density Functional Methods*, Recent Advances in Computational Chemistry, Vol. 1, edited by D. E. Chong (World Scientific, Singapore, 1995) pp. 155–92.
[6] A. D. McLachlan and M. A. Ball, Rev. Mod. Phys. **36**, 844 (1964).
[7] U. von Barth and L. Hedin, J. Phys. C **5**, 1629 (1972).
